# Supplementary material for: VacHopPy: A Python package for vacancy hopping analysis based on molecular dynamics simulations
Source: arXiv:2503.23467 source file (2026-01-09)
Supplement: Supplementary file 1 [file supplementary.pdf]

# Supplementary Material

*VacHopPy*: A Python package for vacancy hopping analysis  
based on *ab initio* molecular dynamics simulations

Taeyoung Jeong<sup>1,2</sup>, Kun Hee Ye<sup>1,2</sup>, Seungjae Yoon<sup>1,2</sup>, Dohyun Kim<sup>1,2</sup>, Yunjae Kim<sup>1,2</sup>, Cheol  
Seong Hwang<sup>2</sup>, and Jung-Hae Choi<sup>\*,1</sup>

<sup>1</sup>*Electronic and Hybrid Materials Research Center, Korea Institute of Science and Technology, Seoul  
02792, Korea*

<sup>2</sup>*Department of Materials Science and Engineering and Inter-University Semiconductor Research  
Center, Seoul National University, Seoul 08826, Korea*

*\*Corresponding author;*

*Tel.: +82 2 958 5488. Fax: +82 2 958 6658*

*E-mail address: choijh@kist.re.kr (J.-H. Choi)*

| Name           | Description                                                                                                                                                                                       |
|----------------|---------------------------------------------------------------------------------------------------------------------------------------------------------------------------------------------------|
| XDATCAR        | <ul style="list-style-type: none"> <li>Information on atomic positions along time (typical VASP output)</li> </ul>                                                                                |
| FORCE          | <ul style="list-style-type: none"> <li>Information on force vectors</li> <li>It can be obtained using the <code>vachoppy -u extract_force</code> command from <code>vasprun.xml</code></li> </ul> |
| OUTCAR         | <ul style="list-style-type: none"> <li>Information of calculation conditions (typical VASP output)</li> </ul>                                                                                     |
| POSCAR_LATTICE | <ul style="list-style-type: none"> <li>POSCAR for a perfect crystalline without vacancy</li> </ul>                                                                                                |

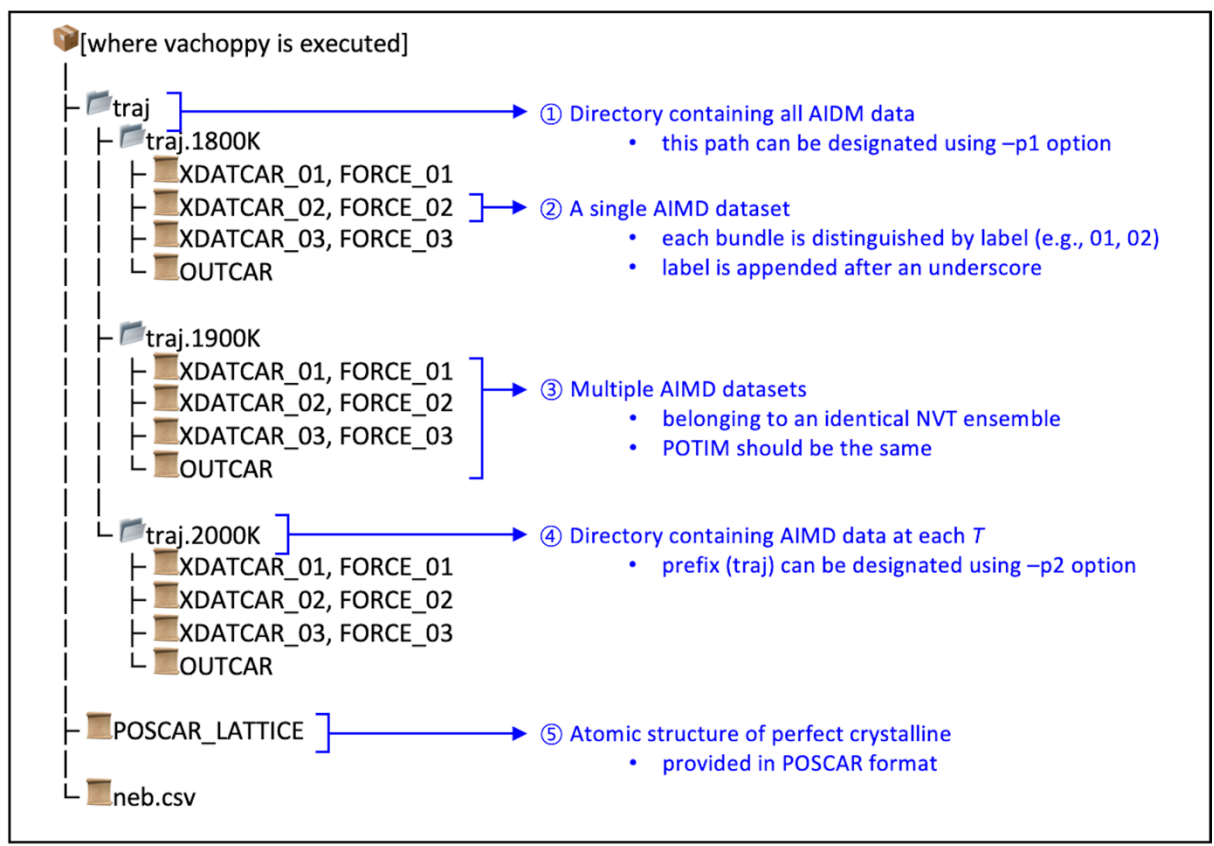

**Figure S1.** Input for AIMD. The upper table summarized the types of input data, while the lower box represents an example file tree. A detailed description and example files are available in the GitHub repository.

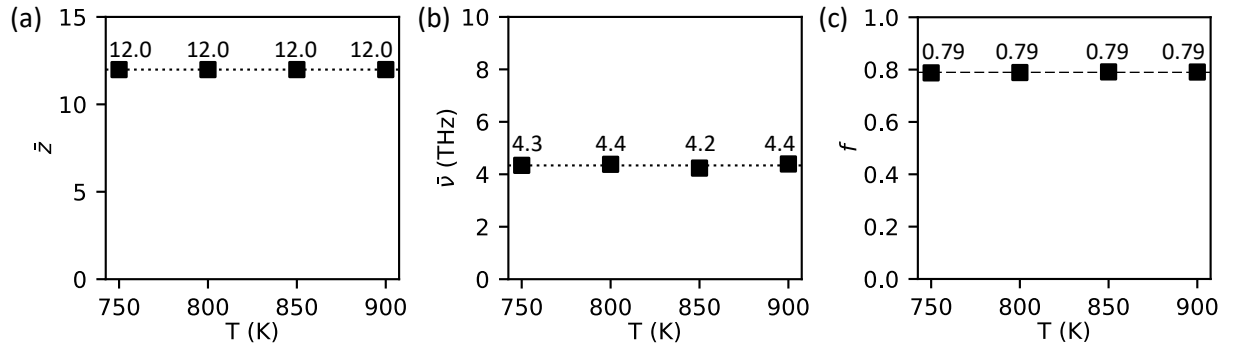

**Figure S2.** *VacHopPy* results for fcc Al. (a)  $\bar{z}$  (b)  $\bar{\nu}$ , and (c)  $f$  as a function of  $T$ , where the dotted lines indicate the mean values.

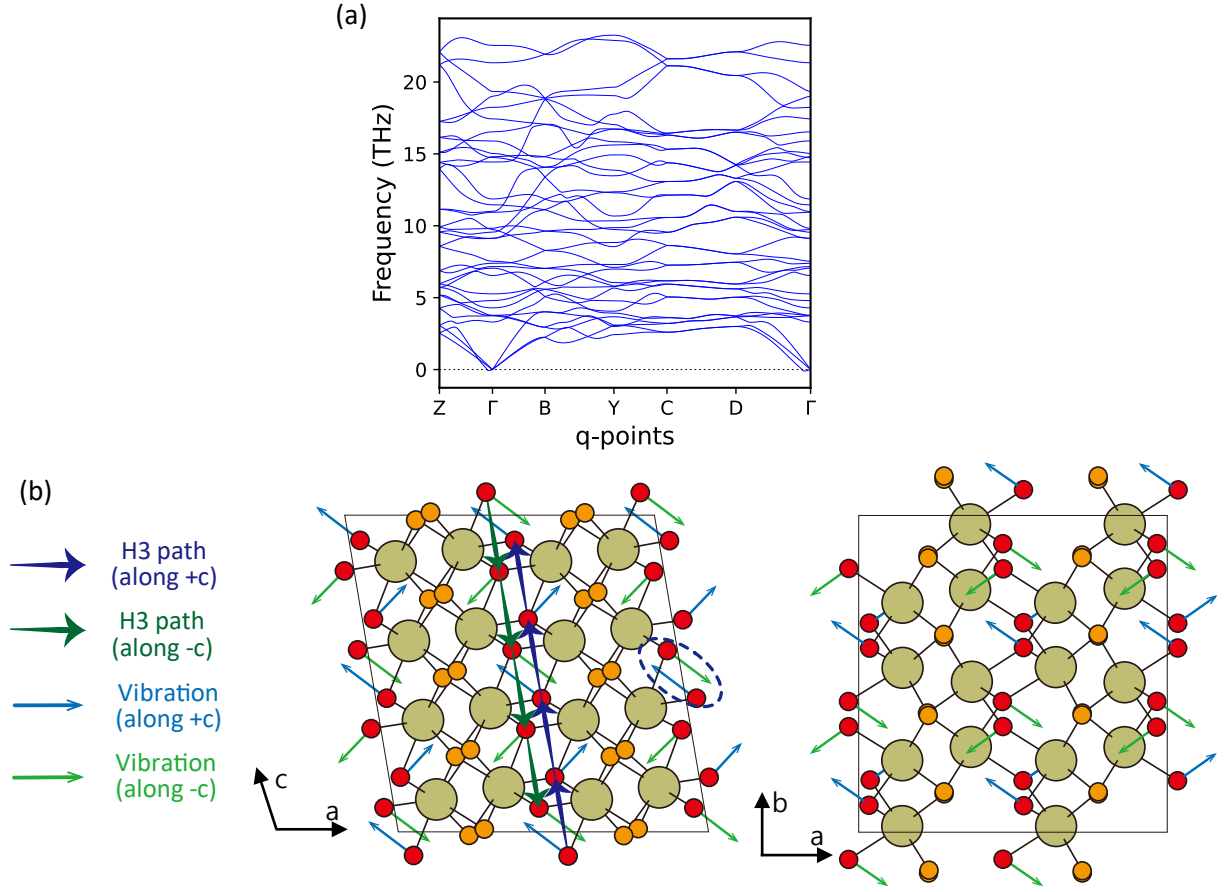

**Figure S3.** (a) Phonon dispersion diagram of monoclinic  $\text{HfO}_2$  (b) Vibration mode corresponding to the lowest optical phonon at  $\Gamma$  point. The vibration direction of each atom is represented by blue (vibration toward +c) and green arrows (vibration toward -c), while the H3 paths are shown together with the thicker blue (along +c) and green arrows (along -c). Note that vector sums of the vibrations with the same color roughly match the H3 path. The description for atoms is the same with Fig. 8 of the main text.

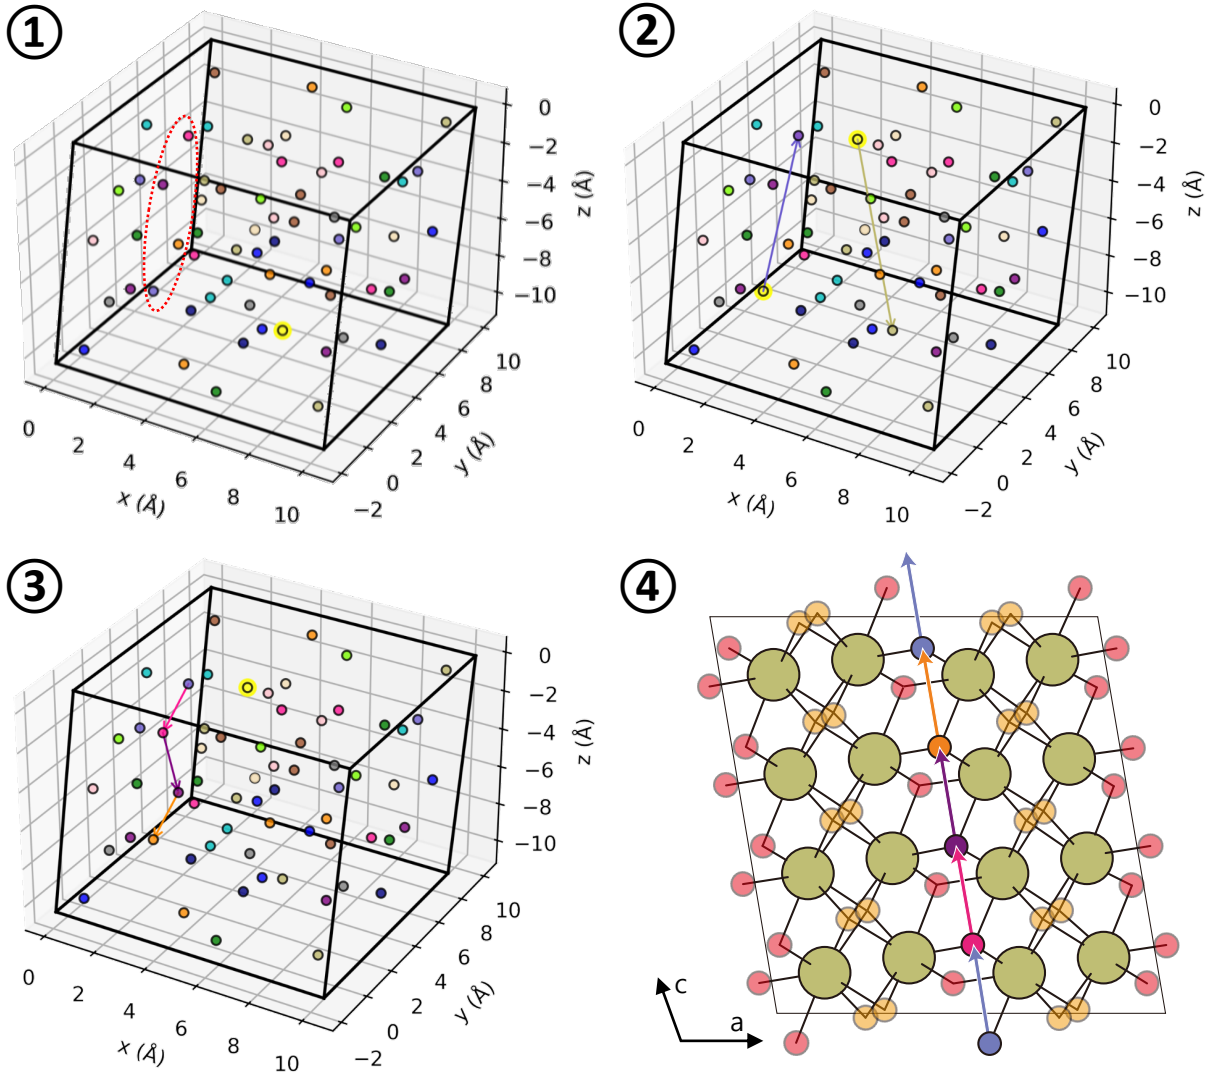

**Figure S4.** Collective movement of 3-coordinated oxygen atoms along the H3 path. The panels ① to ③ show the successive snapshots of the trajectory, obtained using *VacHopPy*, where the four 3-coordinated oxygen atoms (blue, orange, purple, and magenta circles surrounded by the dotted red ellipse) exchange their sites. To help readers understand, this exchange process is summarized in panel ④. The blue, orange, purple, and magenta circles represent the atoms of the same color in the dotted red ellipse of panel ①. These atoms appear to flow along the  $c$ -axis, with all movements along the H3 path represented by arrows.

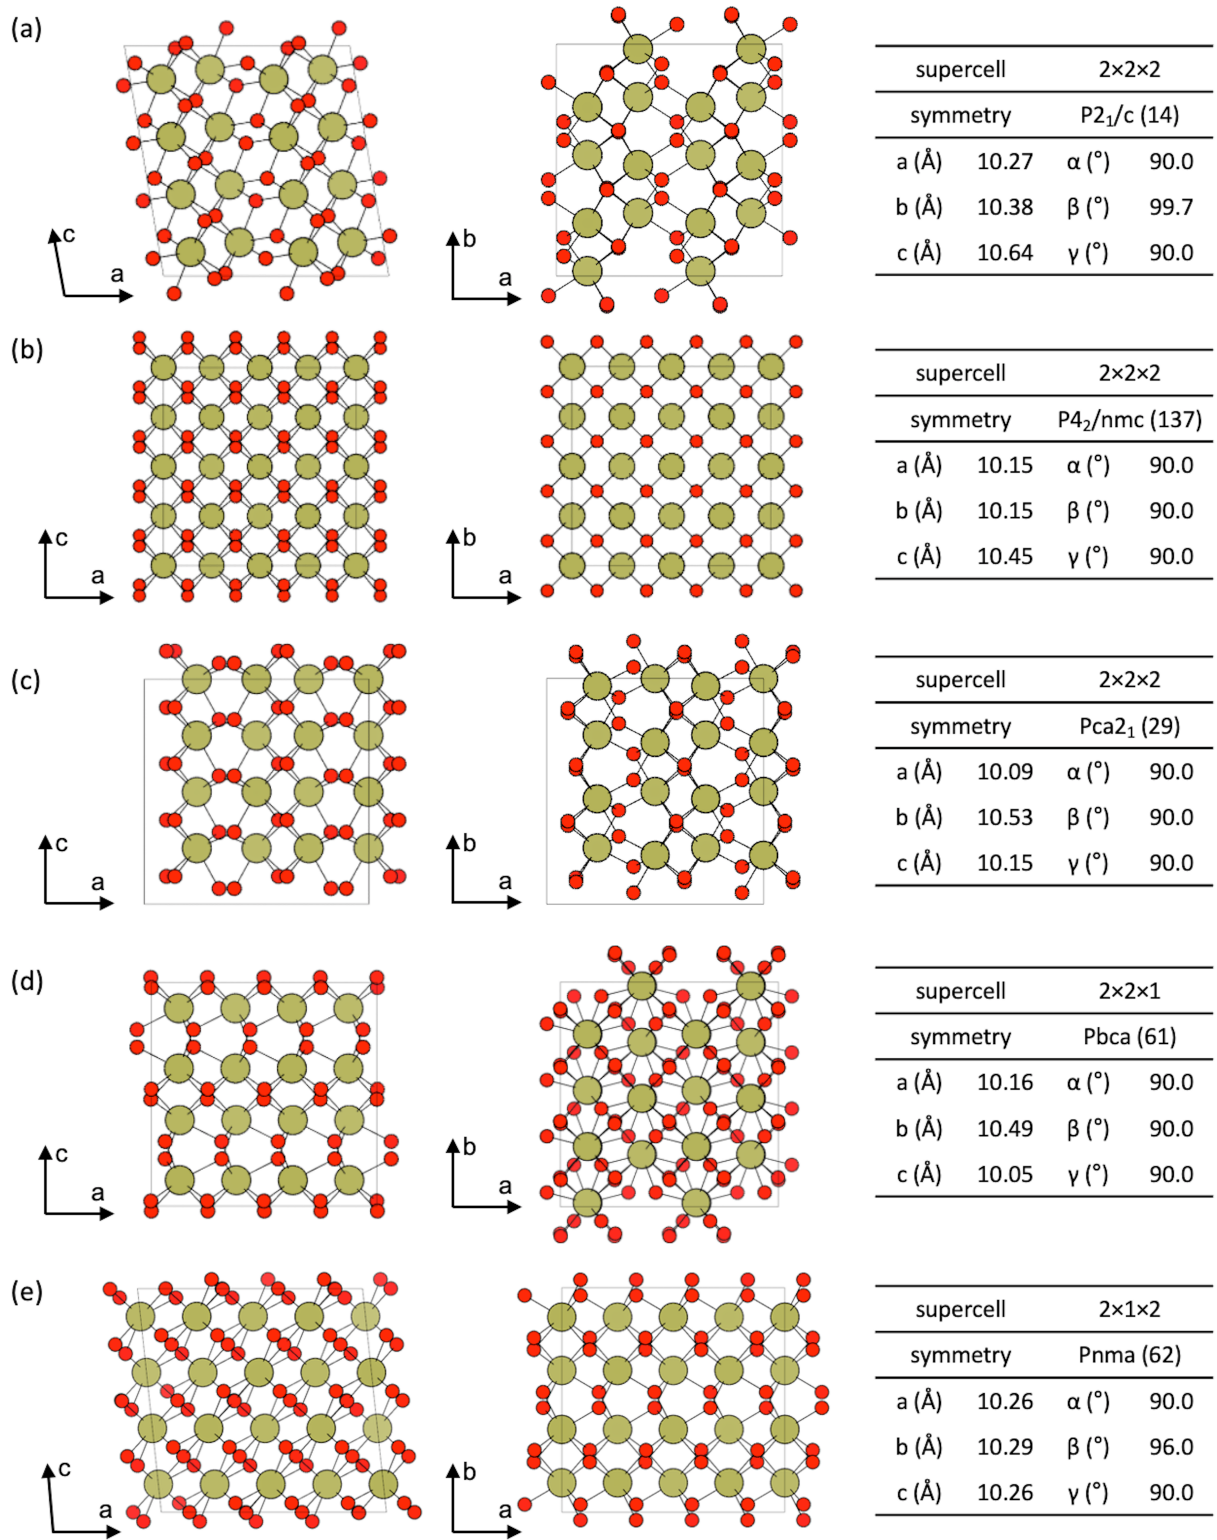

**Figure S5.** Atomic structures of (a) monoclinic (*mono*, P2<sub>1</sub>/c) 2×2×2 supercell, (b) tetragonal (*tet*, P4<sub>2</sub>/nmc) 2×2×2 supercell, (c) polar orthorhombic (*po*, Pca2<sub>1</sub>) 2×2×2 supercell, (d) antipolar orthorhombic (*ao*, Pbca) 2×2×1 supercell, and (e) antipolar orthorhombic (Pnma) 2×1×2 supercell. The Pnma phase is shown in a pseudo-cubic representation for ease of comparison.

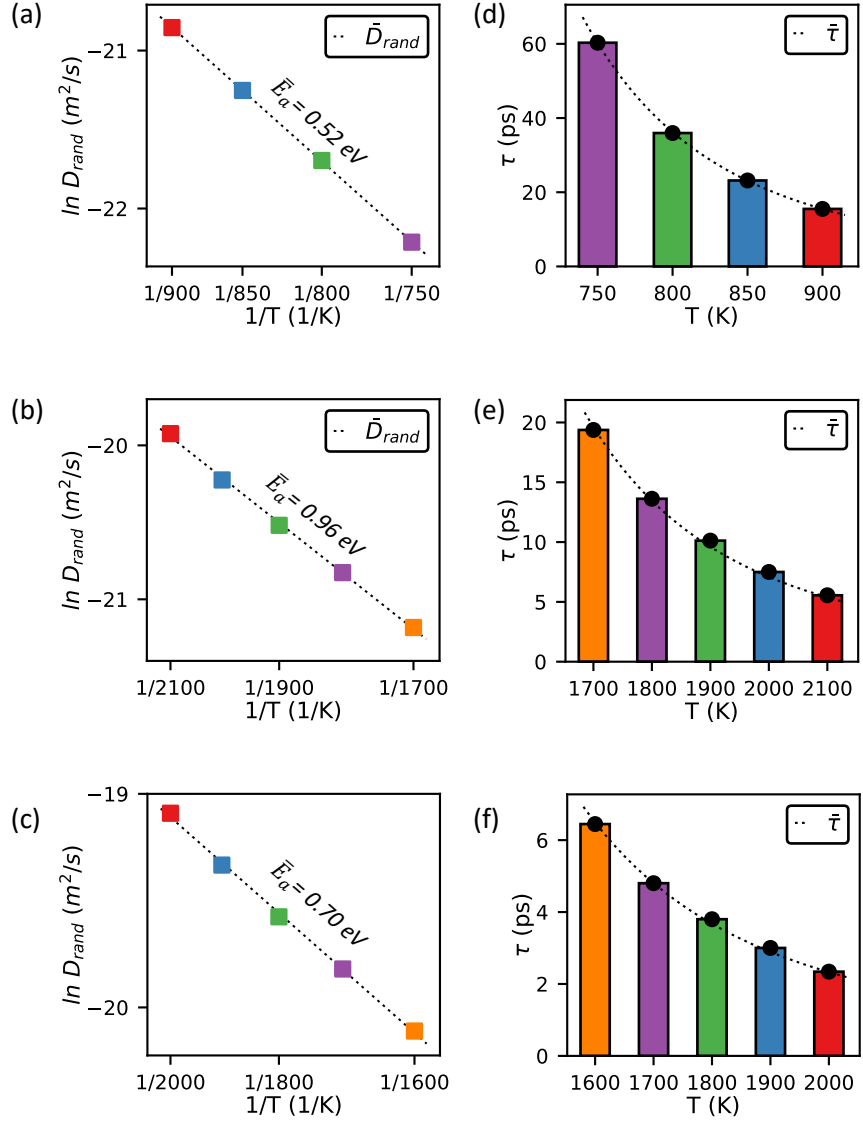

**Figure S6.**  $D_{rand}$  as a function of  $T$  for (a)  $V_{Al}$  in fcc Al, (b)  $V_O^{2+}$  in rutile  $\text{TiO}_2$ , and (c)  $V_O^{2+}$  in monoclinic  $\text{HfO}_2$ . The squares represent the actual  $D_{rand}$  obtained using Eq. (7) of the main text, while the dotted line  $\bar{D}_{rand}$  is obtained using the effective diffusion parameters using Eq. (9) of the main text.  $\tau$  as a function of  $T$  for (d)  $V_{Al}$  in fcc Al, (e)  $V_O^{2+}$  in rutile  $\text{TiO}_2$ , and (f)  $V_O^{2+}$  in monoclinic  $\text{HfO}_2$ . The squares represent the actual  $\tau$  calculated as  $\tau = t/c$ , while the dotted line  $\bar{\tau}$  is obtained using the effective diffusion parameters using Eq. (11) of the main text.

**Table S1.** Notations used in the main text.  $T$ -dependent quantities are denoted by asterisk.

| Notation              | Definition                                                                         | Related equation  |
|-----------------------|------------------------------------------------------------------------------------|-------------------|
| $a$                   | Hopping distance (Å)                                                               |                   |
| $a_{(i,j)}$           | $a$ for $(i, j)$ path (Å)                                                          |                   |
| $\bar{a}$             | Effective $a$ (Å), $\bar{a} = (6\bar{D}_{rand,0}\bar{\tau}_0)^{1/2}$               |                   |
| $c^*$                 | Total number of hopping events                                                     |                   |
| $c_{(i,j)}^*$         | Number of hopping via $(i, j)$ path                                                |                   |
| $c_{enc}^*$           | Average number of vacancy-tracer exchanges per encounter                           | (13)              |
| $D^*$                 | Overall (actual) diffusion coefficient (m <sup>2</sup> /s)                         | (12)              |
| $D_{(i,j)}^*$         | Diffusion coefficient for $(i, j)$ path (m <sup>2</sup> /s)                        | (5)               |
| $D_{rand}^*$          | Overall diffusion coefficient for a random walk process (m <sup>2</sup> /s)        | (6), (7)          |
| $\bar{D}_{rand}^*$    | Effective $D_{rand}$ (m <sup>2</sup> /s)                                           | (9)               |
| $\bar{D}_{rand,0}$    | Pre-exponential factor for $\bar{D}_{rand}$ (m <sup>2</sup> /s)                    | (9)               |
| $d_{cos}(x)$          | Cosine distance from a reference phase $x$                                         | (C.2)             |
| $E_a$                 | Hopping barrier (eV)                                                               |                   |
| $E_{a,(i,j)}$         | $E_a$ for $(i, j)$ path (eV)                                                       |                   |
| $\bar{E}_a$           | Effective $E_a$ (eV)                                                               | (9), (11)         |
| $E_a^f$               | activation energy for $f$                                                          |                   |
| $E_{f,i}$             | vacancy formation energy at $i^{th}$ site (eV)                                     |                   |
| $\mathbf{F}$          | Force (N)                                                                          |                   |
| $f^*$                 | Correlation factor                                                                 | (12), (13), (A.1) |
| $m_i$                 | Number of symmetrically non-equivalent hopping paths at $i^{th}$ site              |                   |
| $\langle m \rangle^*$ | Effective number of hopping path type                                              | (D.4)             |
| $n$                   | Symmetrically non-equivalent vacancy sites                                         |                   |
| $P_i^{site*}$         | Probability that a vacancy resides at $i^{th}$ site                                | (3)               |
| $P_{(i,j)}^*$         | $z_{(i,j)} P_i^{site} P_{(i,j)}^{esc}$                                             | (14)              |
| $P_{(i,j)}^{BD*}$     | Contribution for $(i, j)$ path based on the Boltzmann distribution                 |                   |
| $P_{(i,j)}^{esc*}$    | Escape probability for $(i, j)$ path, $P_{(i,j)}^{esc} = \exp(-E_{a,(i,j)}/k_B T)$ |                   |
| $\bar{P}^{esc*}$      | Effective $P_{(i,j)}^{esc}$                                                        | (15)              |

|                                      |                                                                                                |                   |
|--------------------------------------|------------------------------------------------------------------------------------------------|-------------------|
| $q_{(i,j)}^*$                        | $= c_{(i,j)}/c$                                                                                | (13)              |
| $\langle \mathbf{R}^2 \rangle_{enc}$ | Mean squared displacement of encounters ( $\text{\AA}^2$ )                                     | (13)              |
| $R_{max}$                            | Threshold radius used to construct a fingerprint vector                                        | (C.1)             |
| $t$                                  | Total simulation time of AIMD (ps)                                                             |                   |
| $t_i^*$                              | Total residence time a vacancy stayed at $i^{th}$ site (ps)                                    |                   |
| $t_{interval}$                       | Time interval to be used for averaging (ps)                                                    |                   |
| $z$                                  | Number of equivalent paths                                                                     |                   |
| $z_{(i,j)}$                          | $z$ for $(i,j)$ path                                                                           |                   |
| $\bar{z}^*$                          | Effective $z$ considering all the paths, $\bar{z} = \langle z \rangle \cdot \langle m \rangle$ | (15)              |
| $\langle z \rangle^*$                | Effective $z$ per each $(i,j)$ path                                                            | (D.3)             |
| $\Gamma^*$                           | Overall hopping rate ( $s^{-1}$ )                                                              | (1), (B.1), (B.2) |
| $\Gamma_{(i,j)}^*$                   | Hopping rate via $(i,j)$ path ( $s^{-1}$ )                                                     | (2), (4)          |
| $\Delta$                             | Bin size ( $\text{\AA}$ )                                                                      | (C.1)             |
| $\nu^*$                              | Jump attempt frequency (THz)                                                                   |                   |
| $\nu_{(i,j)}^*$                      | $\nu$ for $(i,j)$ path (THz)                                                                   | (16)              |
| $\bar{\nu}^*$                        | Effective $\nu$ (THz)                                                                          | (14), (B.5)       |
| $\theta_i$                           | Angle between force vector and direction to initial site                                       |                   |
| $\theta_f$                           | Angle between force vector and direction to final site                                         |                   |
| $\rho$                               | Coordinate (or position)                                                                       |                   |
| $\sigma$                             | Standard deviation for Gaussian-smeared delta function                                         | (C.1)             |
| $\tau^*$                             | Overall residence time (ps), $\tau = t/c$                                                      |                   |
| $\bar{\tau}^*$                       | Effective $\tau$ (ps)                                                                          | (11)              |
| $\bar{\tau}_0$                       | Pre-exponential for $\bar{\tau}$ (ps)                                                          | (11)              |

---

**Table 2.** The  $E_a$  values with respect to supercell size.

| $E_a$ from NEB calculations (eV) |      |                 |                 |
|----------------------------------|------|-----------------|-----------------|
| Al                               | Path | 3×3×3 supercell | 4×4×4 supercell |
|                                  | A1   | 0.46            | 0.52            |
| TiO <sub>2</sub>                 | Path | 2×2×3 supercell | 3×3×4 supercell |
|                                  | T1   | 1.04            | 0.87            |
|                                  | T2   | 0.87            | 1.06            |
|                                  | T3   | 1.97            | 1.77            |
| HfO <sub>2</sub>                 | Path | 2×2×2 supercell | 3×3×3 supercell |
|                                  | H1   | 0.71            | 0.68            |
|                                  | H2   | 0.84            | 0.83            |
|                                  | H3   | 0.87            | 0.84            |
|                                  | H4   | 1.37            | 1.31            |
|                                  | H5   | 1.88            | 1.87            |
|                                  | H6   | 2.04            | 2.09            |
|                                  | H7   | 2.00            | 1.99            |
|                                  | F1   | 0.08            | 0.12            |
|                                  | F2   | 0.30            | 0.29            |
|                                  | F3   | 0.86            | 0.79            |
|                                  | F4   | 0.99            | 0.84            |
|                                  | F5   | 1.25            | 1.31            |
|                                  | F6   | 1.41            | 1.52            |
|                                  | F7   | 1.38            | 1.42            |

**Table S3.** Conditions for *ab initio* calculations for each system. Here, the  $N_{cell}$  represents the number of AIMD datasets, which was determined by convergence tests, described in Supplementary note 2.

|                  | POTCAR                        | ENCUT (eV) | k-point | AIMD  |           |            |           | NEB       |
|------------------|-------------------------------|------------|---------|-------|-----------|------------|-----------|-----------|
|                  |                               |            |         | T (K) | Time (ps) | $N_{cell}$ | Supercell | Supercell |
| Al               | PBE<br>(Al)                   | 240.3      | 1×1×1   | 750   | 1200      | 20         | 3×3×3     | 4×4×4     |
|                  |                               |            |         | 800   | 800       | 20         |           |           |
|                  |                               |            |         | 850   | 600       | 20         |           |           |
|                  |                               |            |         | 900   | 400       | 20         |           |           |
| TiO <sub>2</sub> | PBE<br>(Ti <sub>sv</sub> , O) | 400        | 1×1×1   | 1700  | 401       | 20         | 2×2×3     | 3×3×4     |
|                  |                               |            |         | 1800  | 301       | 20         |           |           |
|                  |                               |            |         | 1900  | 251       | 20         |           |           |
|                  |                               |            |         | 2000  | 201       | 20         |           |           |
|                  |                               |            |         | 2100  | 151       | 20         |           |           |
| HfO <sub>2</sub> | PBE<br>(Hf <sub>pv</sub> , O) | 400        | 1×1×1   | 1600  | 200.5     | 20         | 2×2×2     | 3×3×3     |
|                  |                               |            |         | 1700  | 200.5     | 20         |           |           |
|                  |                               |            |         | 1800  | 150.5     | 20         |           |           |
|                  |                               |            |         | 1900  | 200.5     | 20         |           |           |
|                  |                               |            |         | 2000  | 100.5     | 20         |           |           |
|                  |                               |            |         | 2200  | 51        | 3          |           |           |
|                  |                               |            |         | 2400  | 51        | 3          |           |           |
|                  |                               |            |         | 2600  | 51        | 3          |           |           |

### Supplementary note 1. Issues in trajectory determination

Two issues may arise during the trajectory analyses: multi-hopping and multi-vacancy. The multi-hopping issue occurs when two or more consecutive hoppings take place within a single step, as shown in Fig. N1(a). In this example, the vacancy (yellow circle) undergoes two successive hoppings, represented by the magenta (site 1  $\rightarrow$  site 2) and blue (site 2  $\rightarrow$  site 3) arrows. This diagram, generated by *VacHopPy*, uses color-coded circles to represent lattice point occupation by atoms, with the yellow circles indicating unoccupied sites (*i.e.*, vacancies). The arrows show the movement of atoms of the same color. The vacancy moved site 1  $\rightarrow$  site 3 within a single step, but the arrows revealed that the actual path is site 1  $\rightarrow$  site 2  $\rightarrow$  site 3. To correctly interpret such trajectories, *VacHopPy* analyzes the connectivity of the arrows and decomposes consecutive movements automatically. On the other hand, the multi-vacancy issue arises when more than one vacancy is detected, even though the system contains only a single vacancy. It occurs when two atoms are assigned to the same lattice point, creating a transient vacancy. This issue is mainly related to the kick-out mechanism, as shown in Fig. N1(b). In this figure, the blue atom moves from site 1 to site 2, displacing the magenta atom and creating a transient vacancy at site 1 (orange circle). The displaced magenta atom is then kicked out to site 3. As a result, the original vacancy appears to move directly from site 1 to site 3. To identify the original vacancy, *VacHopPy* employs a causal relationship: if the original vacancy has not moved, it should remain at the same site in the previous step. If the vacancy has moved, its final site should be connected to its initial site by the corresponding arrows (e.g., the blue and magenta arrows in Fig. N1(b)). *VacHopPy* resolves this issue automatically, ensuring that only the original vacancy is considered in the trajectory analyses.

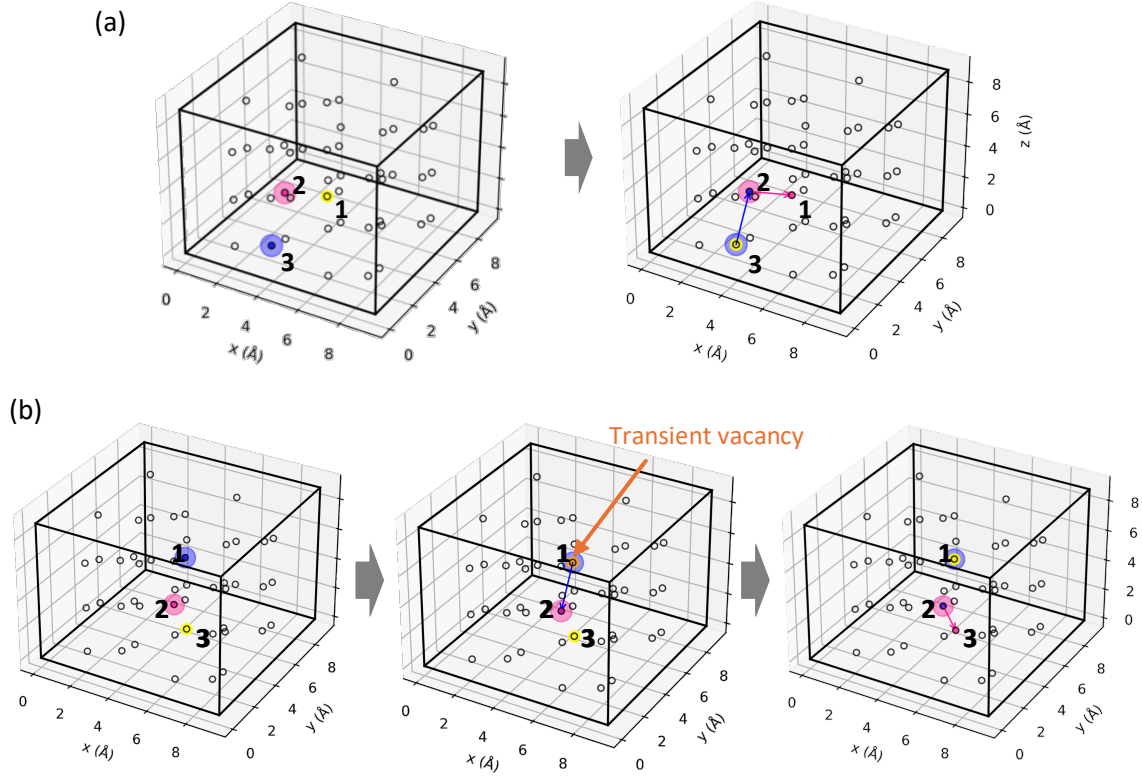

**Figure N1.** Two issues obtained using *VacHopPy*. (a) Multi-hopping issue, where the two panels show successive trajectory snapshots. The yellow circles indicate vacancies, and other circles represent the occupied lattice sites. For clarity, only atoms participating in diffusion are colored by blue and magenta. The transparent backgrounds at lattice sites indicate which atoms were initially presented at those sites. The two-colored arrows in the right panel show the movement of atoms with the same color. Within a single step (or  $t_{interval}$ ), the vacancy at site 1 moved to site 3. However, from the arrows, it can be inferred that the actual vacancy trajectory follows site 1  $\rightarrow$  site 2  $\rightarrow$  site 3. (b) Multi-vacancy issue, where the three panels show successive trajectory snapshots indicating the atomic diffusion via the kick-out mechanism. The blue atom, initially at site 1, moved to site 2, displacing the magenta atom and creating a transient vacancy at site 1 (orange circle). The displaced magenta atom is then kicked out to site 3. As a result, the original vacancy appears to move directly from site 1 to site 3.

## Supplementary note 2. Hyperparameter determination

Determining an appropriate set of hyperparameters is crucial for the reliable implementation of *VacHopPy*. Key hyperparameters include AIMD simulation time ( $t$ ), the number of cells used in AIMD simulations ( $N_{cell}$ ), and the time interval for averaging the simulation data ( $t_{interval}$ ). Based on the author's experience, the parameter  $t$  should be long enough to ensure each AIMD simulation captures at least 20 hopping events for reliable analyses. Hence, running AIMD simulations at high temperature ( $T$ ) can reduce the calculation burden. The proper  $N_{cell}$  and  $t_{interval}$  can be determined through a convergence test of  $f$  with respect to these parameters, as  $f$  is related to key quantities such as mean squared displacement (MSD) and the count of each hopping path ( $c_{(i,j)}$ ). Examples of the convergence tests are provided below for three systems: face-centered cubic (fcc) Al, rutile TiO<sub>2</sub>, and monoclinic HfO<sub>2</sub>.

### 2.1 Fcc Al

Fig. N2(a) shows the convergence of  $f$  as a function of  $N_{cell}$ . The  $f$  values converge at  $N_{cell} = 20$ ; thereby, 20 cells were employed for AIMD simulations at each  $T$ . Similarly, Fig. N2(b) shows the convergence of  $f$  with respect to  $t_{interval}$ , with the  $f$  values converging at  $t_{interval} = 0.1$  ps (dotted line). Fig. N2(c) compares the convergence of  $f$  with and without considering force vectors. The force vectors are used to understand the distribution of the transition state (TS), as described in Section 2.1 of the main text. Accordingly, in the case with force vectors, the trajectory of vacancy was determined based on TS criteria, whereas in the case without force vectors, the trajectory was determined based on proximity alone. While the  $f$  values converge to the same value in both cases, use of force vectors results in faster convergence, demonstrating that TS criteria can enhance reliability of calculations.

## 2.2 Rutile TiO<sub>2</sub>

The convergence tests to determine hyperparameters in the rutile TiO<sub>2</sub> system are shown in Fig. N3. Similar to fcc Al, Fig. N3(a) represents the convergence of  $f$  with respect to  $N_{cell}$ , while Fig. N3(b) shows the  $f$  values as a function of  $t_{interval}$ . The results confirm that  $f$  converges at  $N_{cell} = 20$  and  $t_{interval} = 0.1$  ps.

## 2.3 Monoclinic HfO<sub>2</sub>

Fig. N4(a) shows  $f$  values as a function of  $T$  for the monoclinic HfO<sub>2</sub> system. The result confirms that convergence of  $f$  is achieved at  $N_{cell} = 20$ . Fig. N4(b) represents the convergence of  $f$  with respect to  $t_{interval}$ . However, the  $f$  values do not converge but instead continuously increase as  $t_{interval}$  increases, with the abrupt decrease in slope observed at  $t_{interval} = 0.05$  ps. This behavior highlights a limitation of *VacHopPy* trajectory analysis: return processes that occur within a single step are not detectable since atomic positions are captured step by step. Specifically, during trajectory determination of monoclinic HfO<sub>2</sub>, some return processes involving successive movement through the H1 and F1 paths may be omitted. This occurs because the return process is rapid due to the significantly low  $E_a$  of the F1 path and the energetic instability of the F-site. As  $t_{interval}$  increases, more return processes may be disregarded, leading to a reduction in  $c_{enc}$  in Eq. (13) of the main text and, consequently, an increase in  $f$ . To address this issue, the total count of hopping events, excluding hoppings via the H1 and F1 paths, was used as an alternative to  $f$ . As shown in Fig. N4(c), the convergence is nearly achieved at  $t_{interval} = 0.05$  ps, consistent with the decrease in slope observed in Fig. N4(b).

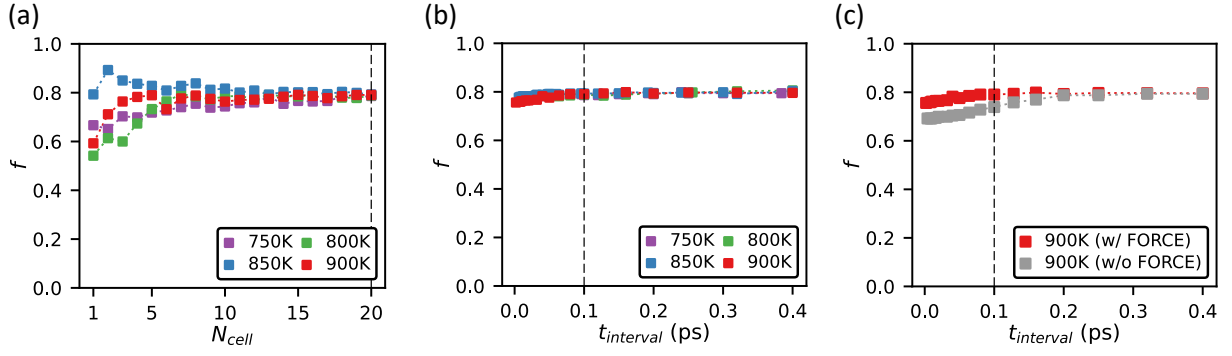

**Figure N2.** Convergence tests based on  $f$  for fcc Al. The  $f$  is converged at (a)  $N_{cell} = 20$  (b)  $t_{interval} = 0.1$  ps. (c) Comparison convergence of  $f$  with (red) and without (grey) the TS refinement using force vectors at 900 K. Using TS refinement achieves faster convergence.

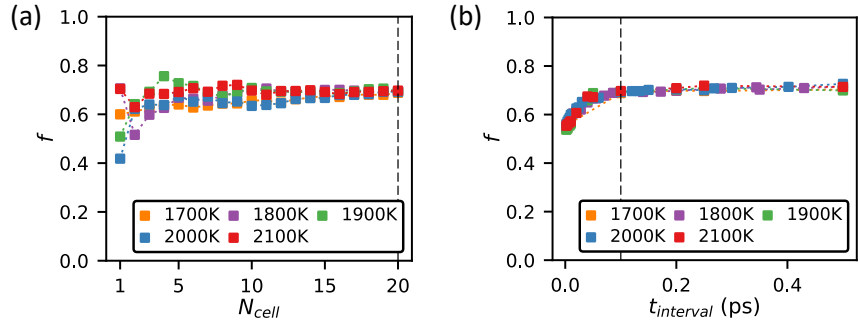

**Figure N3.** Convergence tests based on  $f$  for rutile  $TiO_2$ . The  $f$  is converged at (a)  $N_{cell} = 20$  (b)  $t_{interval} = 0.1$  ps.

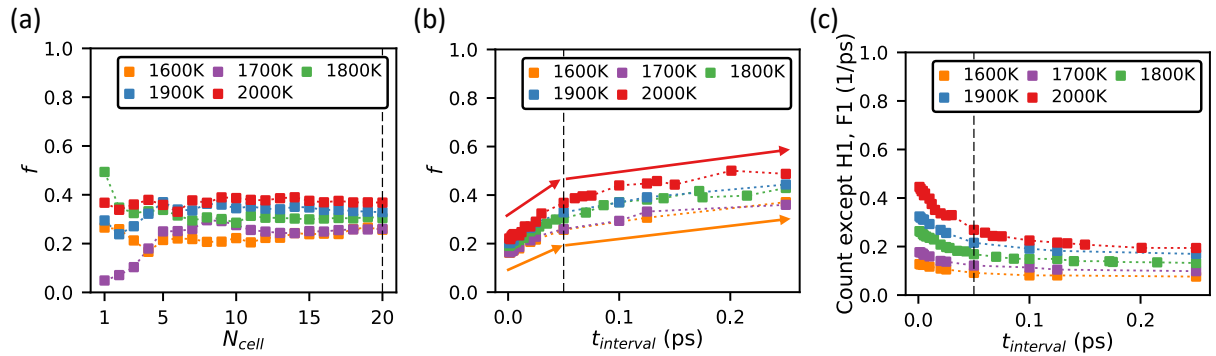

**Figure N4.** Convergence tests for monoclinic  $HfO_2$ . (a) The  $f$  is converged at  $N_{cell} = 20$ . (b) For  $t_{interval}$ ,  $f$  does not converge but continuously increase with  $t_{interval}$ . However, an obvious decrease in slop is observed at  $t_{interval} = 0.05$  ps (dotted line). (c) Convergence test on  $t_{interval}$  based on the total count of hopping events, excluding hops via the H1 and F1 paths, instead of  $f$ . Convergence is nearly achieved at  $t_{interval} = 0.05$  ps (dotted line).

### Supplementary note 3: Jump attempt frequency from the Eyring's formula

Eyring's formula is given by [1]:

$$\nu = \frac{k_B T}{h} \exp\left(-\frac{\Delta E_{vib}}{k_B T}\right) \quad (\text{N. 1})$$

where  $\Delta E_{vib}$  is the difference in vibrational free energy between the initial and transition states of a hopping path, and  $k_B$  is the Boltzmann constant. For the following examples, the phonon data was obtained using the same conditions with the NEB calculations shown in Table S3. The vibrational free energy calculations were performed using Phonopy [2] using  $21 \times 21 \times 21$  k-meshes.

#### 3.1 Fcc Al

Figs. N5(a) and (b) show the phonon dispersions for the initial and the transition state of the Al path in fcc Al, respectively. Some imaginary phonon modes are detected in these diagrams, which are excluded from the vibrational free energy calculations. Hence, the presence of the imaginary phonon can undermine the reliability of the  $\nu$  calculation. The flat imaginary phonon indicated by an arrow in Fig. N5(b) is associated with the hopping process. The calculated  $\nu$  values are shown in Fig. N5(c) as a function of  $T$ . The yellow region indicates the simulated  $T$  region. Within the simulated  $T$  region,  $T$ -dependence of  $\nu$  is insignificant, and the mean  $\nu$  value is found to be 3.0 THz.

#### 3.2 Rutile TiO<sub>2</sub>

Fig. N6(a) represents the phonon dispersion of the rutile TiO<sub>2</sub> conventional cell (without  $V_O^{2+}$ ).

Under our calculation conditions, the rutile  $\text{TiO}_2$  appears to be kinetically unstable, as several imaginary phonons are observed. Furthermore, Figs. N6(b) and (c) show the phonon dispersions for the initial and the transition states of the T2 path, respectively, obtained from the  $3 \times 3 \times 4$  supercell. A number of imaginary phonons are present, including a phonon associated with the hopping process, which appears as a flat line in the imaginary region in Fig. N6(c). The vibrational free energies were calculated using these phonon dispersions, and the resulting  $\nu$  value obtained using Eq. (N1) is shown in Fig. N6(d) as a function of  $T$ . The mean  $\nu$  value within the simulated  $T$  range was found to be  $1.2 \times 10^{12}$  THz, far exceeding the typical range of 1-10 THz. This discrepancy is likely due to the presence of abundant imaginary phonons in Figs. N6(b) and (c), which can hamper the accuracy of the vibrational free energy calculations.

### 3.3 Monoclinic $\text{HfO}_2$

For the monoclinic  $\text{HfO}_2$  system, five major hopping paths, the H1, H2, H3, F1, and F2 paths, are considered. The phonon dispersion diagrams for the initial and the transition states corresponding to each path, as well as the  $\nu$  values as a function of  $T$ , are shown in Fig. N7. While the phonons of the conventional monoclinic  $\text{HfO}_2$  cell without  $\text{V}_0^{2+}$  are stable (as shown in Fig. S3(a)), a few imaginary phonons appear in all phonon dispersion diagrams in Fig. N7, likely originating from lattice distortion induced by  $\text{V}_0^{2+}$ . Compared to the rutile  $\text{TiO}_2$  system, the influence of imaginary phonons is expected to be less significant, as their number is relatively small, and their appearances are similar between the initial and transition states. The flat phonon branches observed in the phonon dispersions of each transition state are responsible for the hopping process.

However, the exact impact of the imaginary phonons (except for the flat phonon branches) remains unclear. For example, as shown in the right panel of Fig. N7(c), the  $T$ -dependence of  $\nu$  exhibits an inverse trend compared to general expectation, with higher  $\nu$  values at lower  $T$ . For all considered paths, the  $T$ -dependence of  $\nu$  is negligible within the simulated  $T$  range.

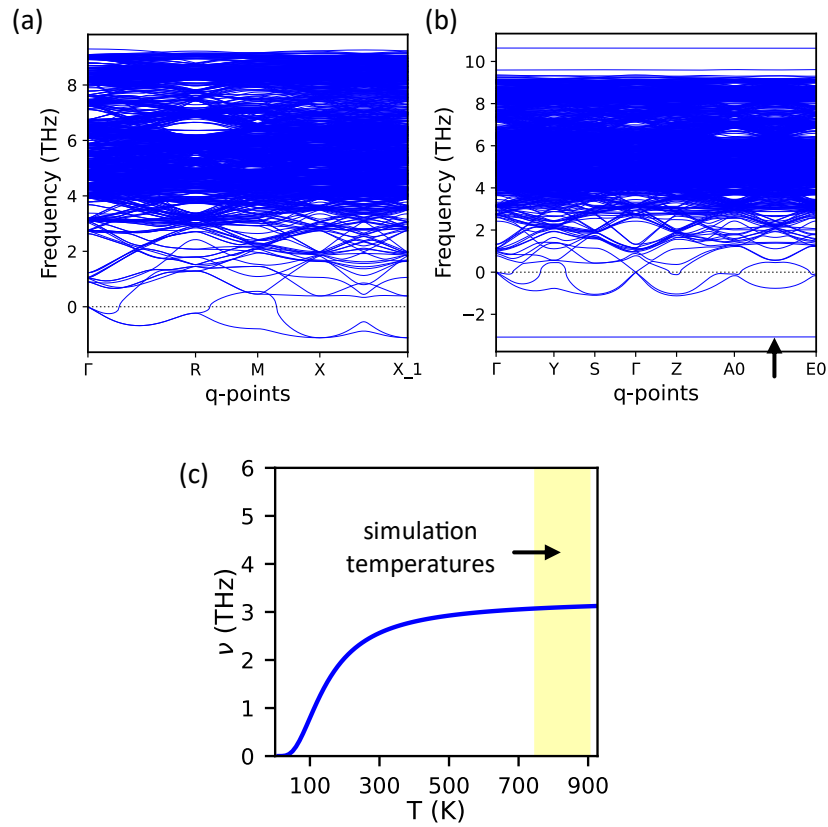

**Figure N5.** Phonon dispersion diagrams of the (a) initial and (b) transition states for Al path in fcc Al, respectively. The flat phonon branch in (b), indicated by an arrow, is associated to the hopping process. (c)  $\nu$  as a function of  $T$ , which was obtained using the Eyring's formula. The yellow region indicates the simulated  $T$  range.

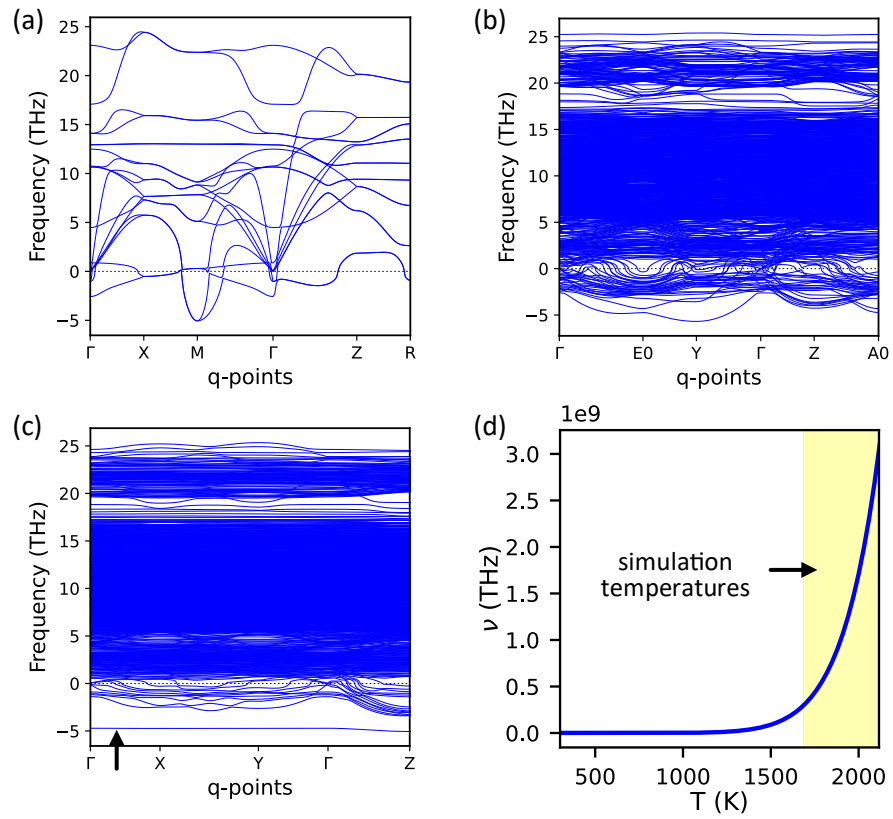

**Figure N6.** (a) Phonon dispersion rutile  $\text{TiO}_2$  conventional cell under our calculation conditions. Phonon dispersion diagrams of the (b) initial state and (c) transition state of the T2 path. The phonon branch associated to the hopping process is indicated by an arrow in (c). (d)  $\nu$  as a function of  $T$ , which was obtained using the Eyring's formula. The yellow region indicates the simulated  $T$  range.

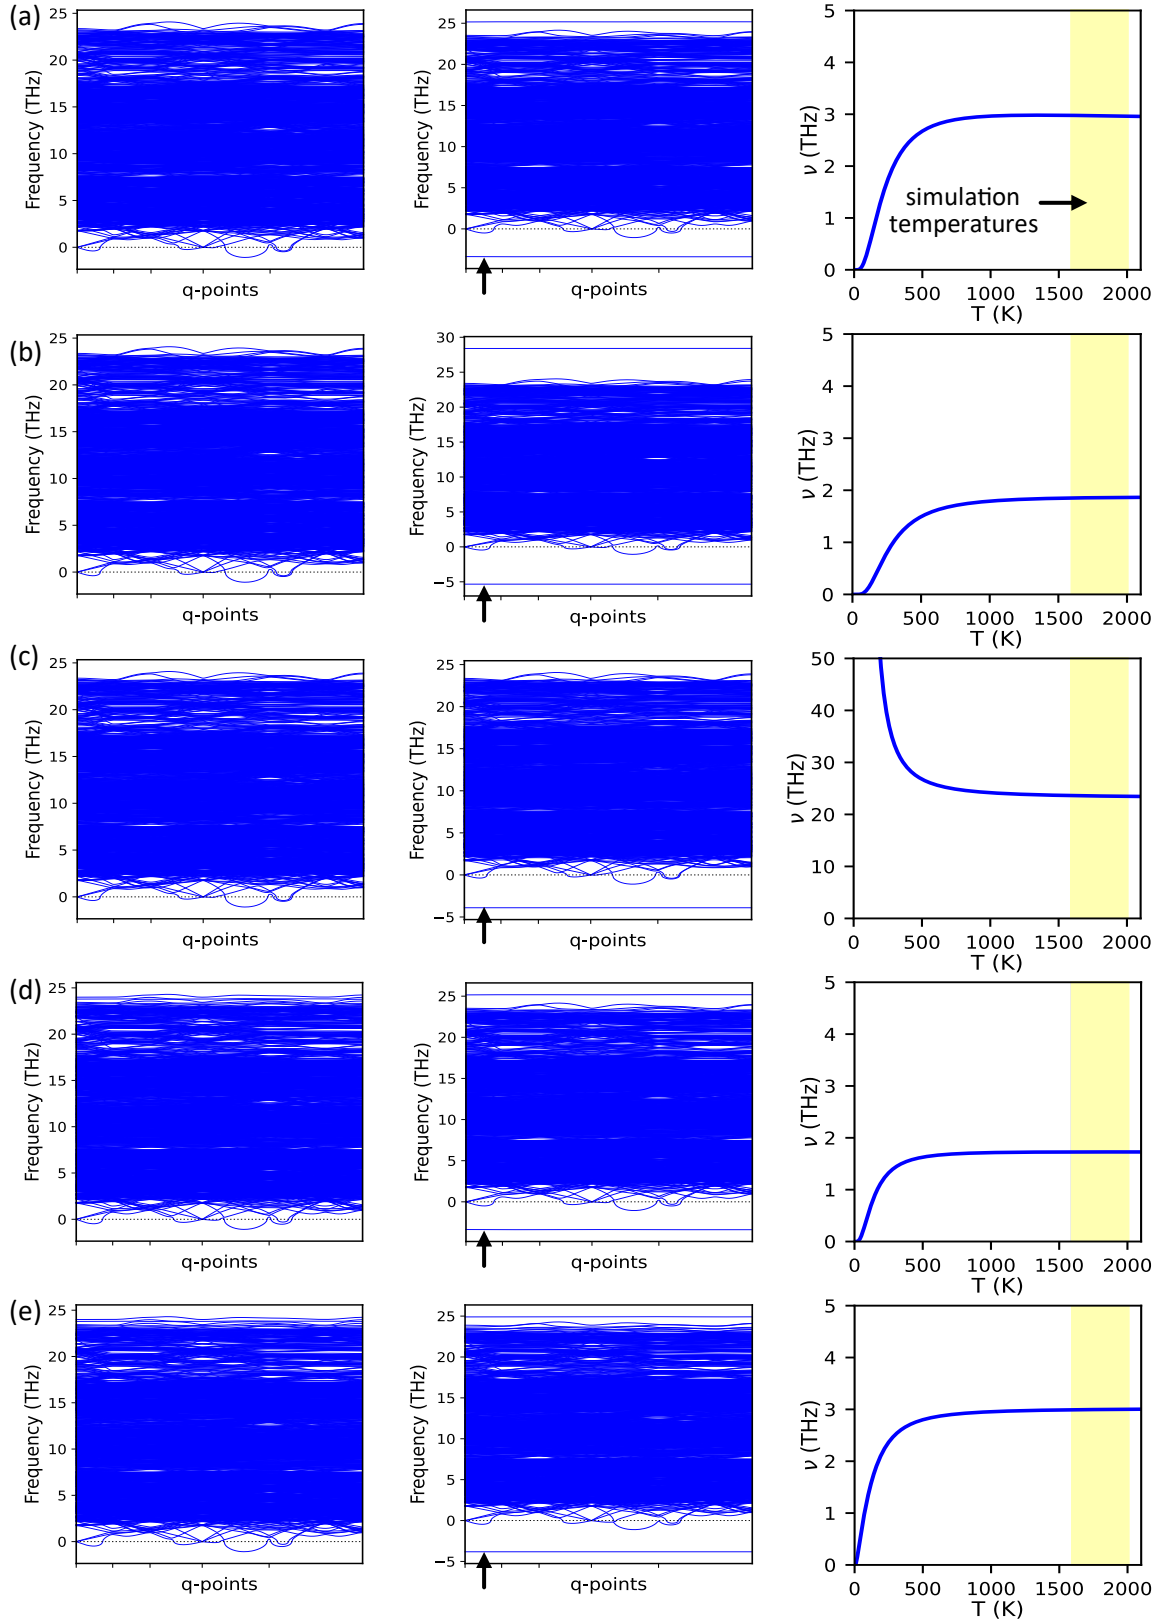

**Figure N7.** Phonon dispersion diagrams for the initial state (left panel) and transition states (middle panel) for the (a) H1 path (b) H2 path (c) H3 path (d) F1 path, and (e) F2 path, respectively. In the middle panel, the phonon branches associated with the hopping process are indicated by arrows. The right panels show the corresponding  $\nu$  as a function of  $T$ , obtained using the Eyring's formula, where the yellow regions indicate the simulated  $T$  range.

## Reference

- [1] Henry Eyring. The activated complex and the absolute rate of chemical reactions. *Chemical Reviews*, 17(1):65–77, 1935.
- [2] Atsushi Togo, First-principles Phonon Calculations with Phonopy and Phono3py, *Journal of the Physical Society of Japan*, 92:012001, 2023.
